# Supplementary material for: Quantum thermodynamics of integrable and near-integrable atomic systems
Source: arXiv:2410.16771 source file (2024-10-22)
Supplement: Supplementary file 1 [file Appendix.tex]

% ***************************************************
% Appendix
% ***************************************************
\chapter{Appendix}

\subsection{Normal modes}\label{Chap:2_Sec:NormalModes}
We first note that the dressing operation, given by
\begin{equation}
    f^\mathrm{dr}(\theta) = f(\theta) + \int \frac{d \lambda}{2 \pi} \varphi(\theta - \lambda) n(\lambda) f^\mathrm{dr}(\lambda),
\end{equation}
may be expressed in terms of integral operators as
\begin{equation}
    f^\mathrm{dr}= f + \varphi N f^\mathrm{dr},
\end{equation}
where $N$ and $n$ are integral operators over the rapidity, defined through
\begin{equation}
    N f = \int d\lambda n(\theta) \delta(\theta-\lambda) f_s(\lambda) = n(\theta)  f_s(\lambda)
\end{equation}
\begin{equation}
    \varphi f = \int d\lambda \varphi(\theta - \lambda)  f_s(\lambda) 
\end{equation}
We note that we have overloaded the definition of $\varphi$, yet this will not pose a problem, as the function $\varphi(\theta)$ does not occur in this appendix.

We may thus express any dressed function through rearranging and inverting this functional relation, as
\begin{equation}
    f^\mathrm{dr} = (1 - \varphi N)^{-1} f.
\end{equation}
Through this, we may express the density of states from the TBA as, 
\begin{equation}\label{eq}
    f_s = 1^\mathrm{dr} =  (1 - \varphi N)^{-1} 1.
\end{equation}
Further, we see simply that
\begin{equation}\label{eq:p'_condition}
    f_p = N(1 - \varphi N)^{-1} p',
\end{equation}
\begin{equation}\label{eq:E'_condition}
     v^\mathrm{eff} f_p = N(1 - \varphi N)^{-1} E'.
\end{equation}

Next, we may utilize the following expansion of integral operators, which may be considered as a ordinary Taylor expansion,
\begin{equation}
    N(1-\varphi N)^{-1} = N(1 + \varphi N + \varphi N \varphi N + ...) = N + N\varphi N + N \varphi N \varphi N + ...
\end{equation}
Differentiating any term in this series with respect to $u = x$ or $t$, find simply
\begin{equation}
    \partial_u (N \varphi N \varphi N \cdots) = \partial_u(N) \varphi N \varphi N \cdots + N \varphi \partial_u(N) \varphi N + ...
\end{equation}
giving the simple final results
\begin{equation}\label{eq:operator_derivative}
    \partial_u\left(N(1-\varphi N)^{-1}\right) = (1-N\varphi)^{-1} (\partial_u N) (1-\varphi N)^{-1}.
\end{equation}
Combining these results with our hydrodynamic formula
\begin{equation}
    \partial_t(2\pi f_p) + \partial_z(2 \pi v^\mathrm{eff} f_p) = \partial_t \left( N(1-\varphi N)^{-1} p' \right) + \partial_z \left( N(1-\varphi N)^{-1} E' \right) = 0,
\end{equation}
where we used Eq's \ref{eq:p'_condition} and \ref{eq:E'_condition}. This equation is then equivalent, by Eq.~\ref{eq:operator_derivative}, to
\begin{equation}
    (1-N\varphi)^{-1} \partial_t N (1-\varphi N)^{-1} p' + (1-N\varphi)^{-1} \partial_z N (1-\varphi N)^{-1} E' = 0.
\end{equation}
Finally, acting on the left with $(1-N \varphi)$ and utilizing the dressing function and the definition of the effective velocity, we arrive at the final equation
\begin{equation}
    \partial_t n + v^\mathrm{eff}[n] \partial_z n = 0.
\end{equation}
